# Supplementary material for: SDRT: Enhance Vision-Language Models by Self-Distillation with Diverse Reasoning Traces
Source: arXiv:2503.01754 source file (2025-03-19)
Supplement: Supplementary file 2 [file 10_preliminary.tex]

\section{Preliminary Experiments}
\label{sec:preliminary}
