# Supplementary material for: SDRT: Enhance Vision-Language Models by Self-Distillation with Diverse Reasoning Traces
Source: arXiv:2503.01754 source file (2025-03-19)
Supplement: Supplementary file 3 [file 11_ablation.tex]

\section{Ablation Study}
