# Supplementary material for: SDRT: Enhance Vision-Language Models by Self-Distillation with Diverse Reasoning Traces
Source: arXiv:2503.01754 source file (2025-03-19)
Supplement: Supplementary file 4 [file 12_analysis.tex]

\section{Qualitative Analysis}
